# Supplementary material for: FDS: Frequency-Aware Denoising Score for Text-Guided Latent Diffusion Image Editing
Source: arXiv:2503.19191 source file (2025-03-24)
Supplement: Supplementary file 1 [file figs-supp.pdf]

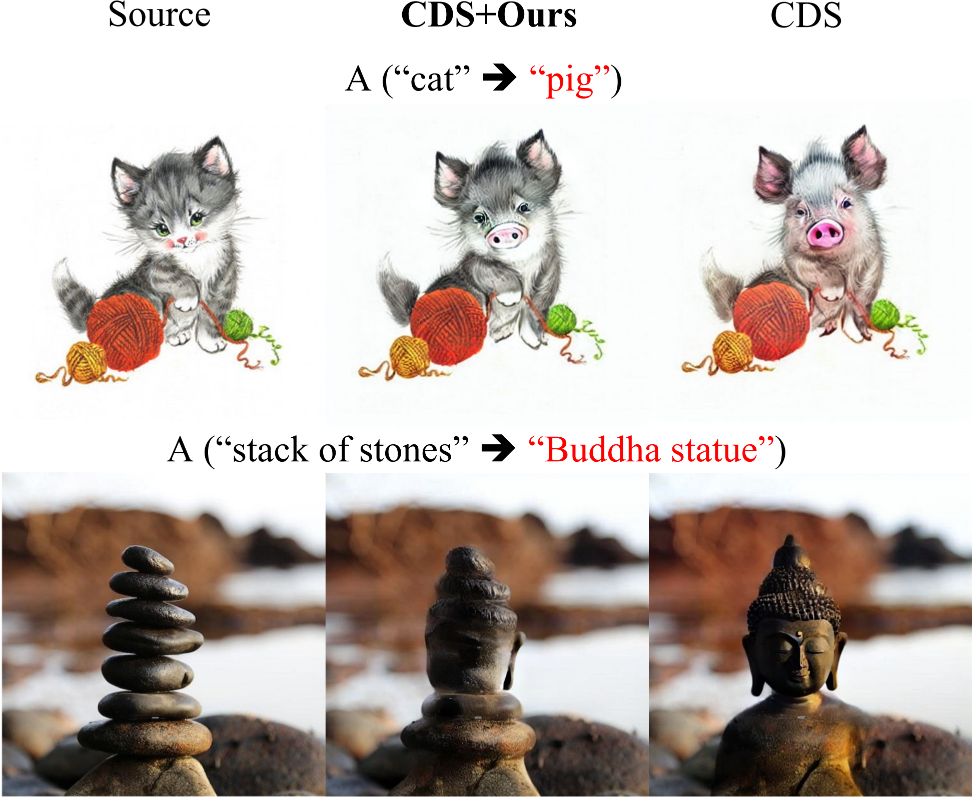
Source
CDS+Ours
CDS
A (“cat” ➔ “pig”)
A (“stack of stones” ➔ “Buddha statue”)

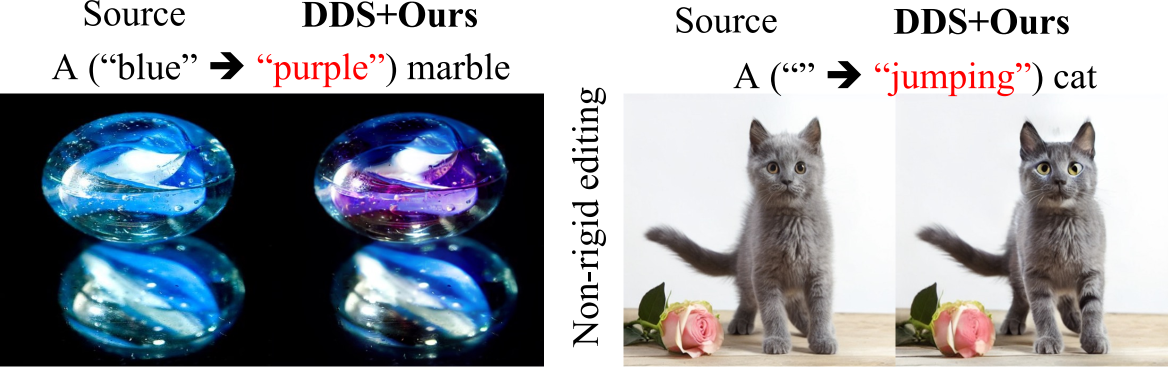


(a) Understanding reflection (b) Non-rigid editing

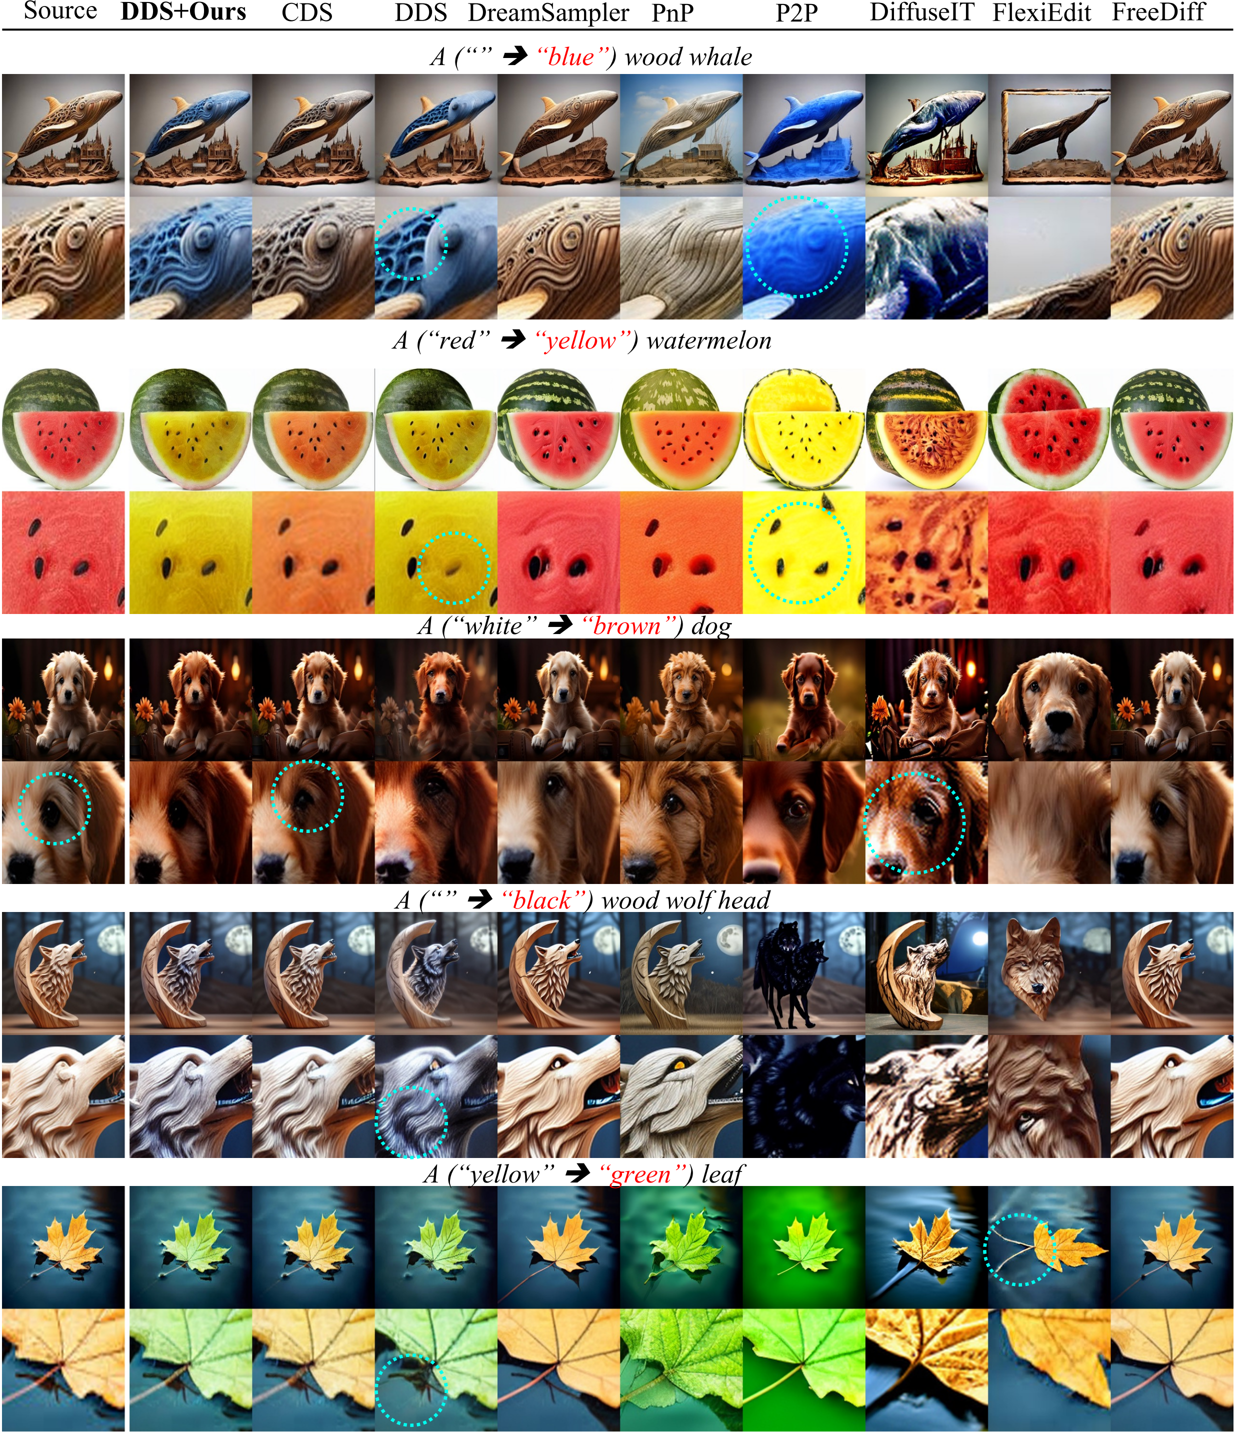
Source
DDS+Ours
CDS
DDS
DreamSampler
PnP
P2P
DiffuseIT
FlexiEdit
FreeDiff
A ("" ➔ "blue") wood whale
A ("red" ➔ "yellow") watermelon
A ("white" ➔ "brown") dog
A ("" ➔ "black") wood wolf head
A ("yellow" ➔ "green") leaf

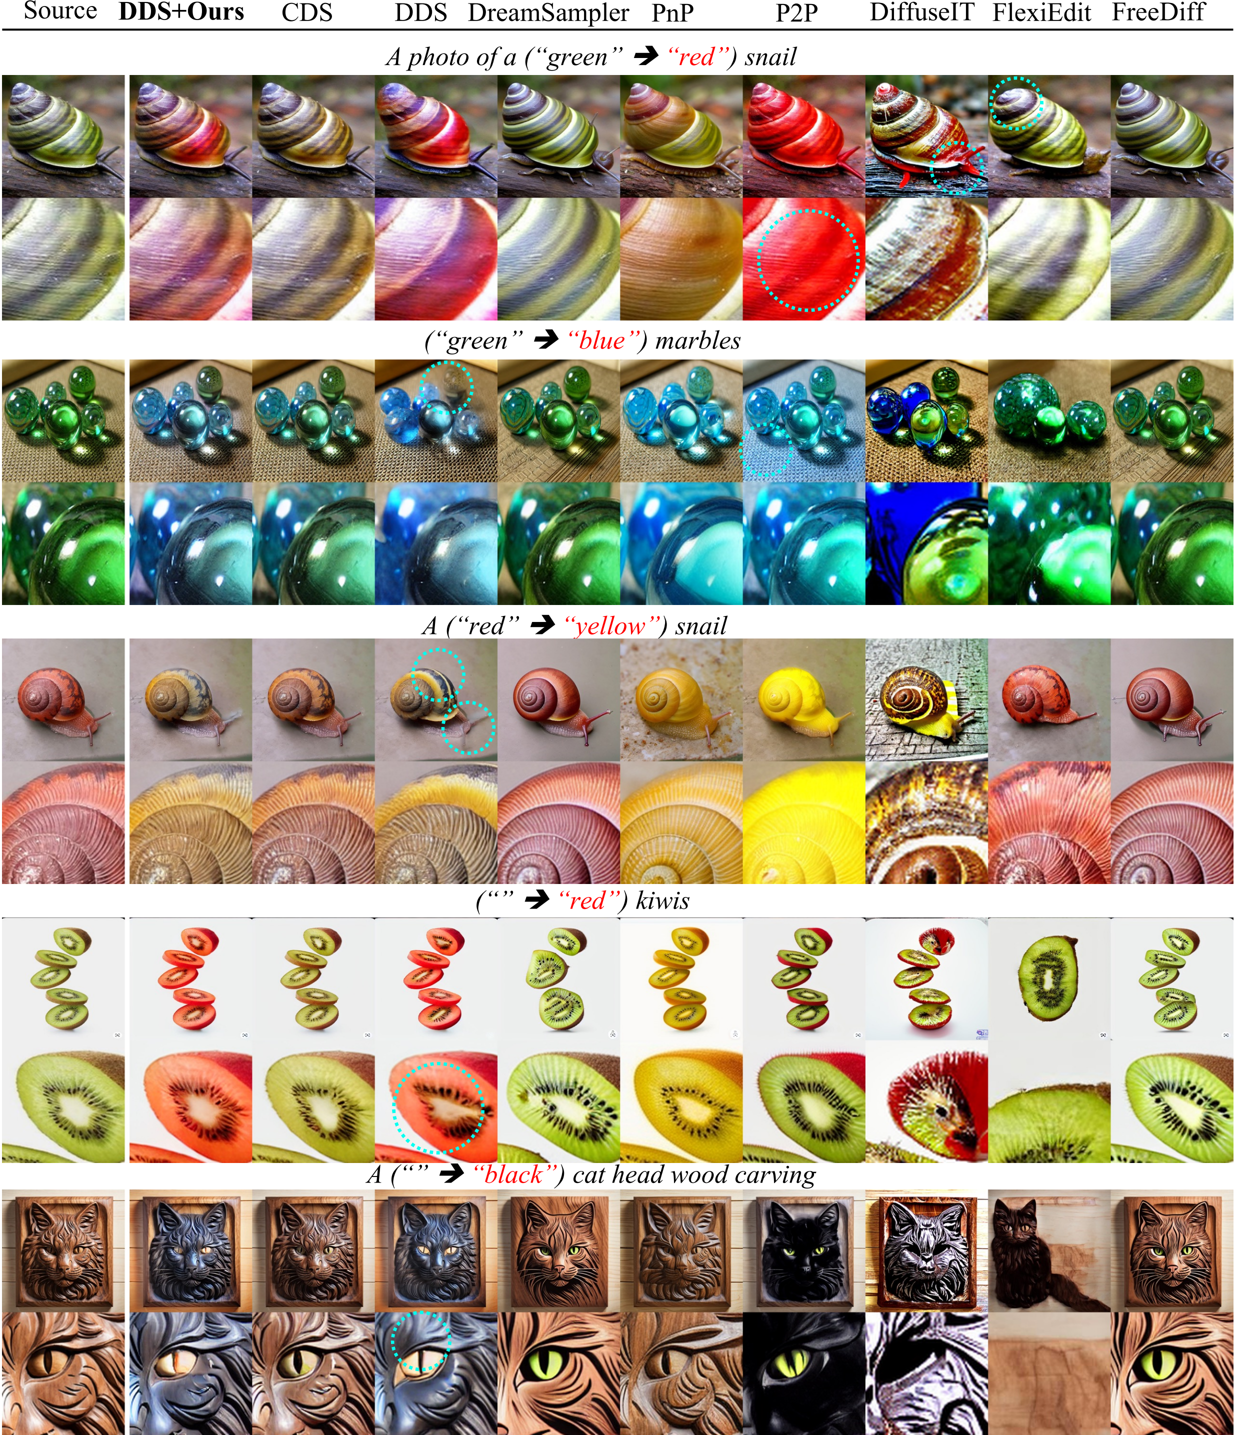
Source
DDS+Ours
CDS
DDS
DreamSampler
PnP
P2P
DiffuseIT
FlexiEdit
FreeDiff
A photo of a ("green" ➔ "red") snail
("green" ➔ "blue") marbles
A ("red" ➔ "yellow") snail
("" ➔ "red") kiwis
A ("" ➔ "black") cat head wood carving

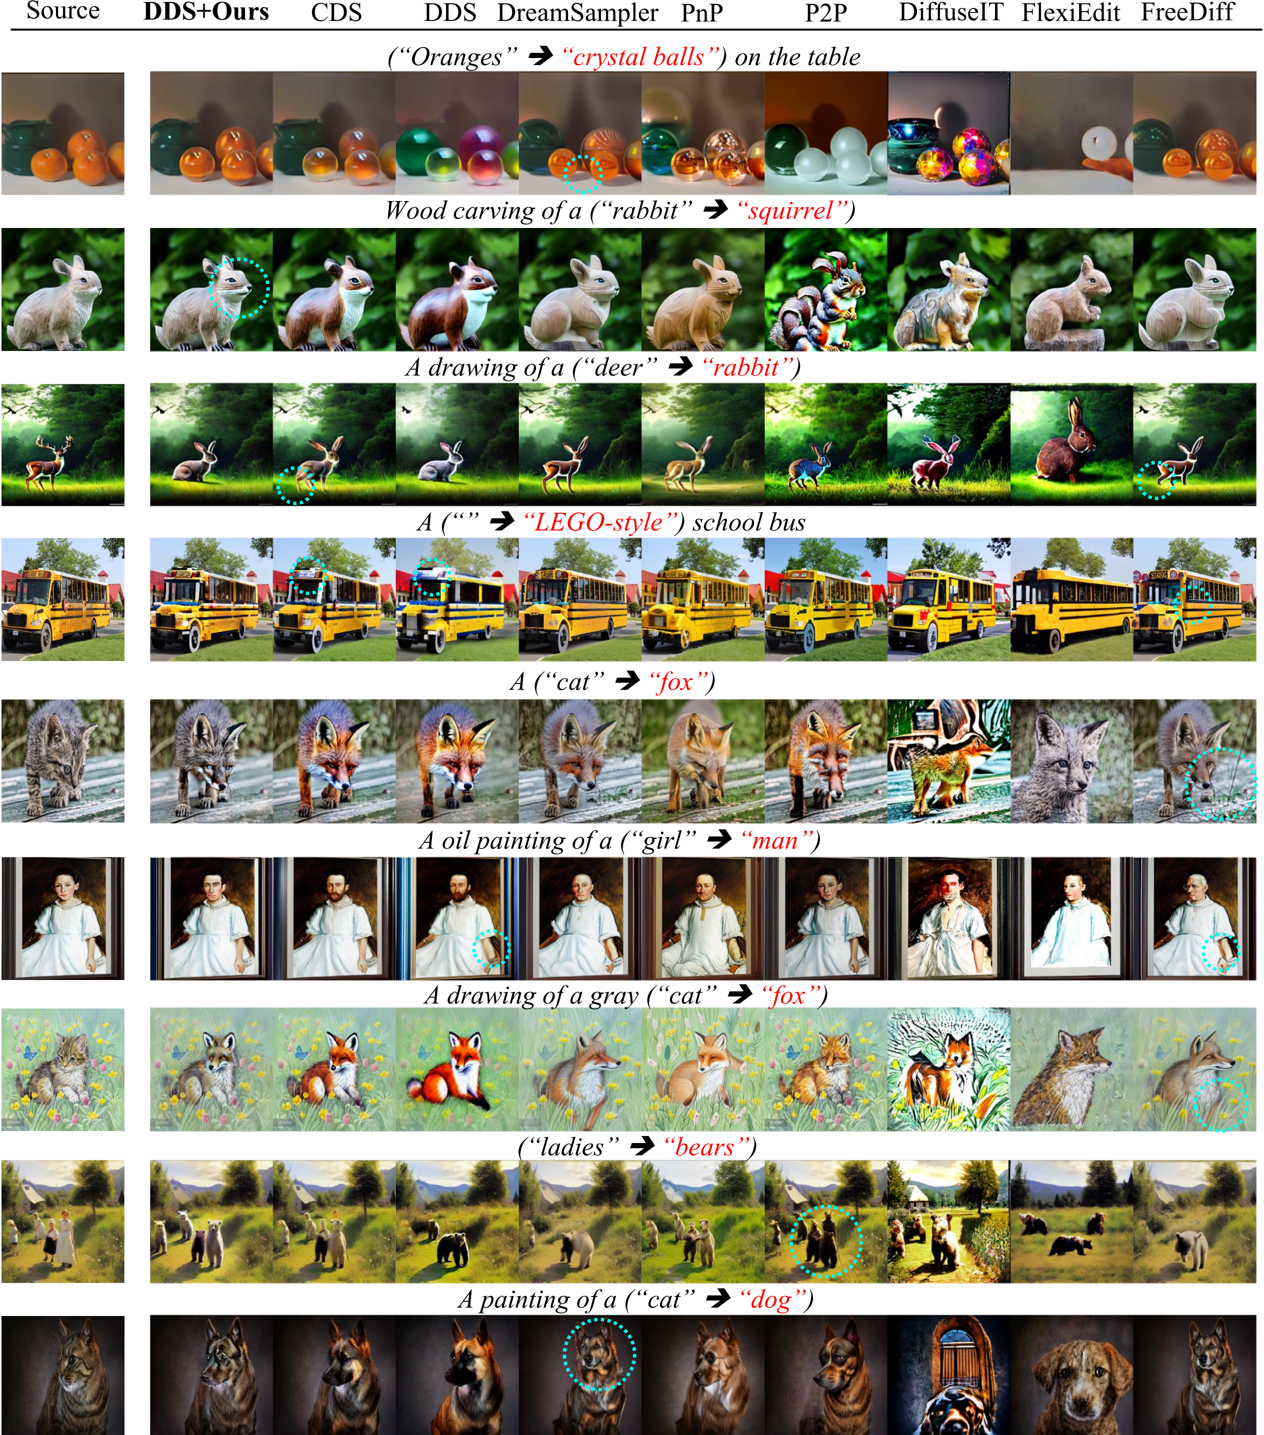
Source
DDS+Ours
CDS
DDS
DreamSampler
PnP
P2P
DiffuseIT
FlexiEdit
FreeDiff
(“Oranges” ➔ “crystal balls”) on the table
Wood carving of a (“rabbit” ➔ “squirrel”)
A drawing of a (“deer” ➔ “rabbit”)
A (“” ➔ “LEGO-style”) school bus
A (“cat” ➔ “fox”)
A oil painting of a (“girl” ➔ “man”)
A drawing of a gray (“cat” ➔ “fox”)
(“ladies” ➔ “bears”)
A painting of a (“cat” ➔ “dog”)

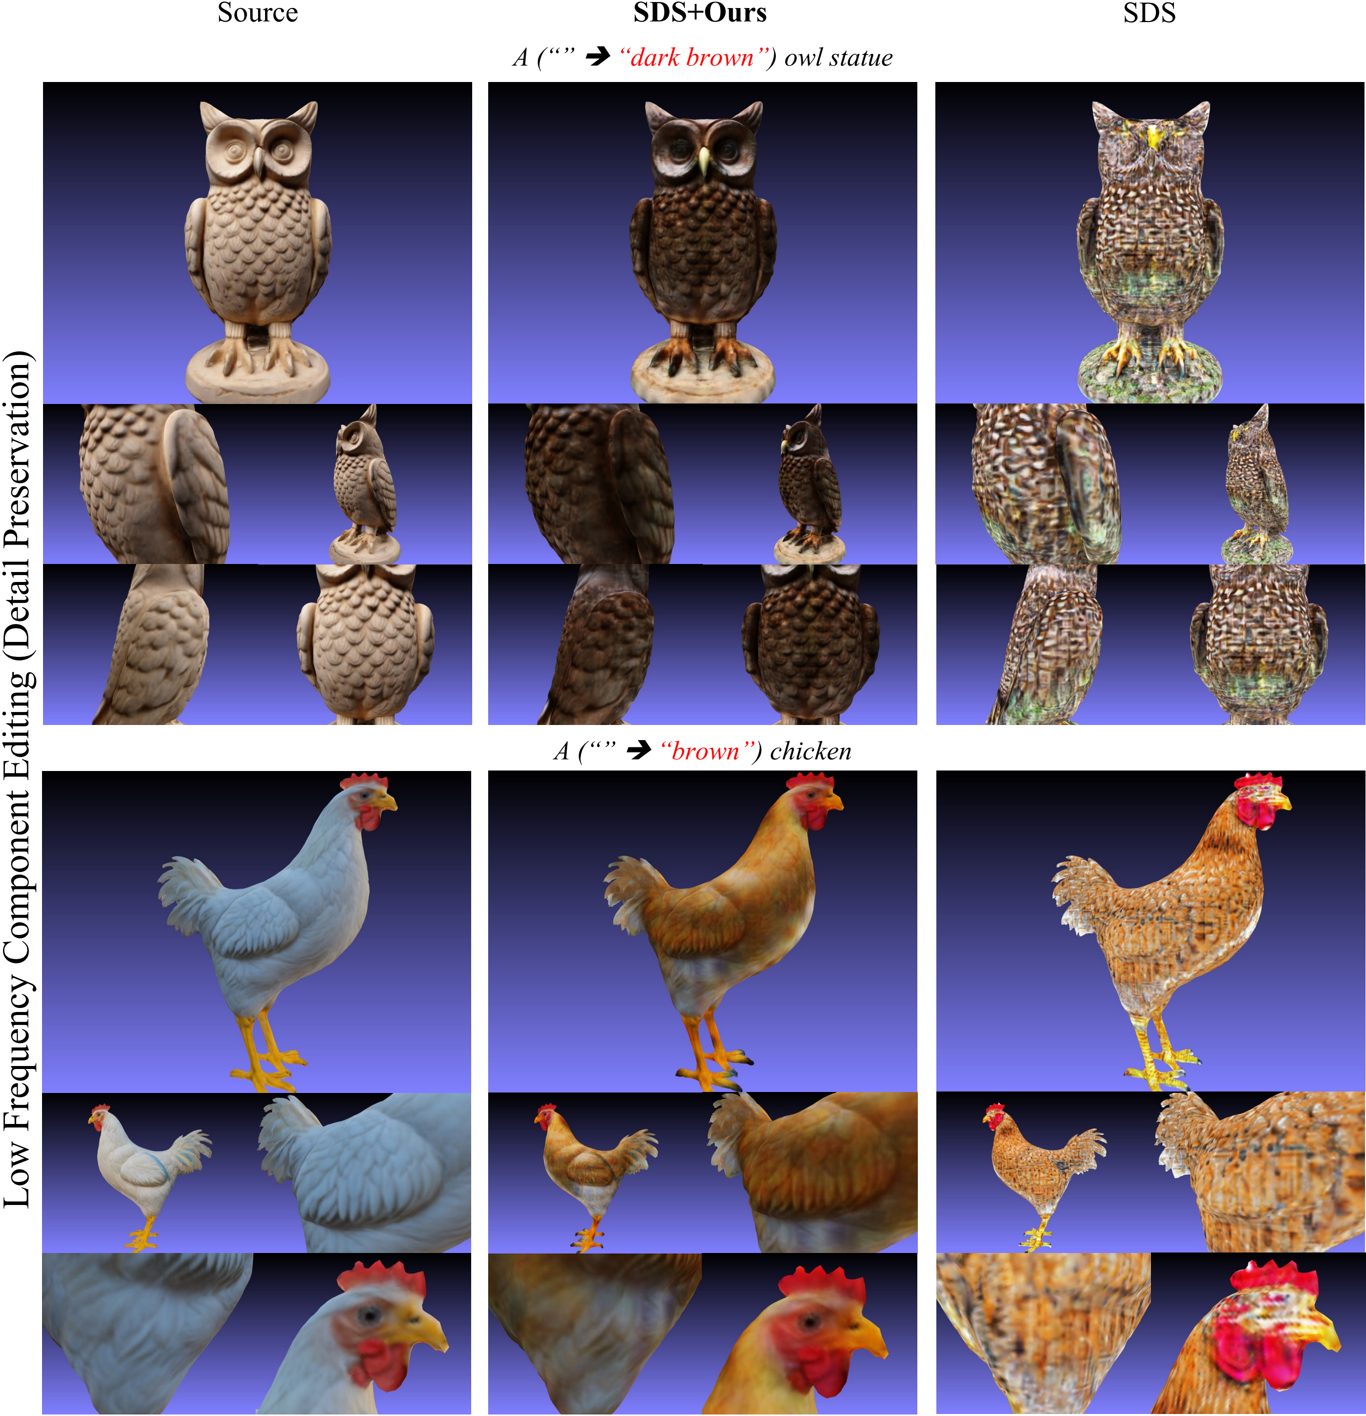
Source
SDS+Ours
SDS
A ("" ➔ "dark brown") owl statue
A ("" ➔ "brown") chicken
Low Frequency Component Editing (Detail Preservation)

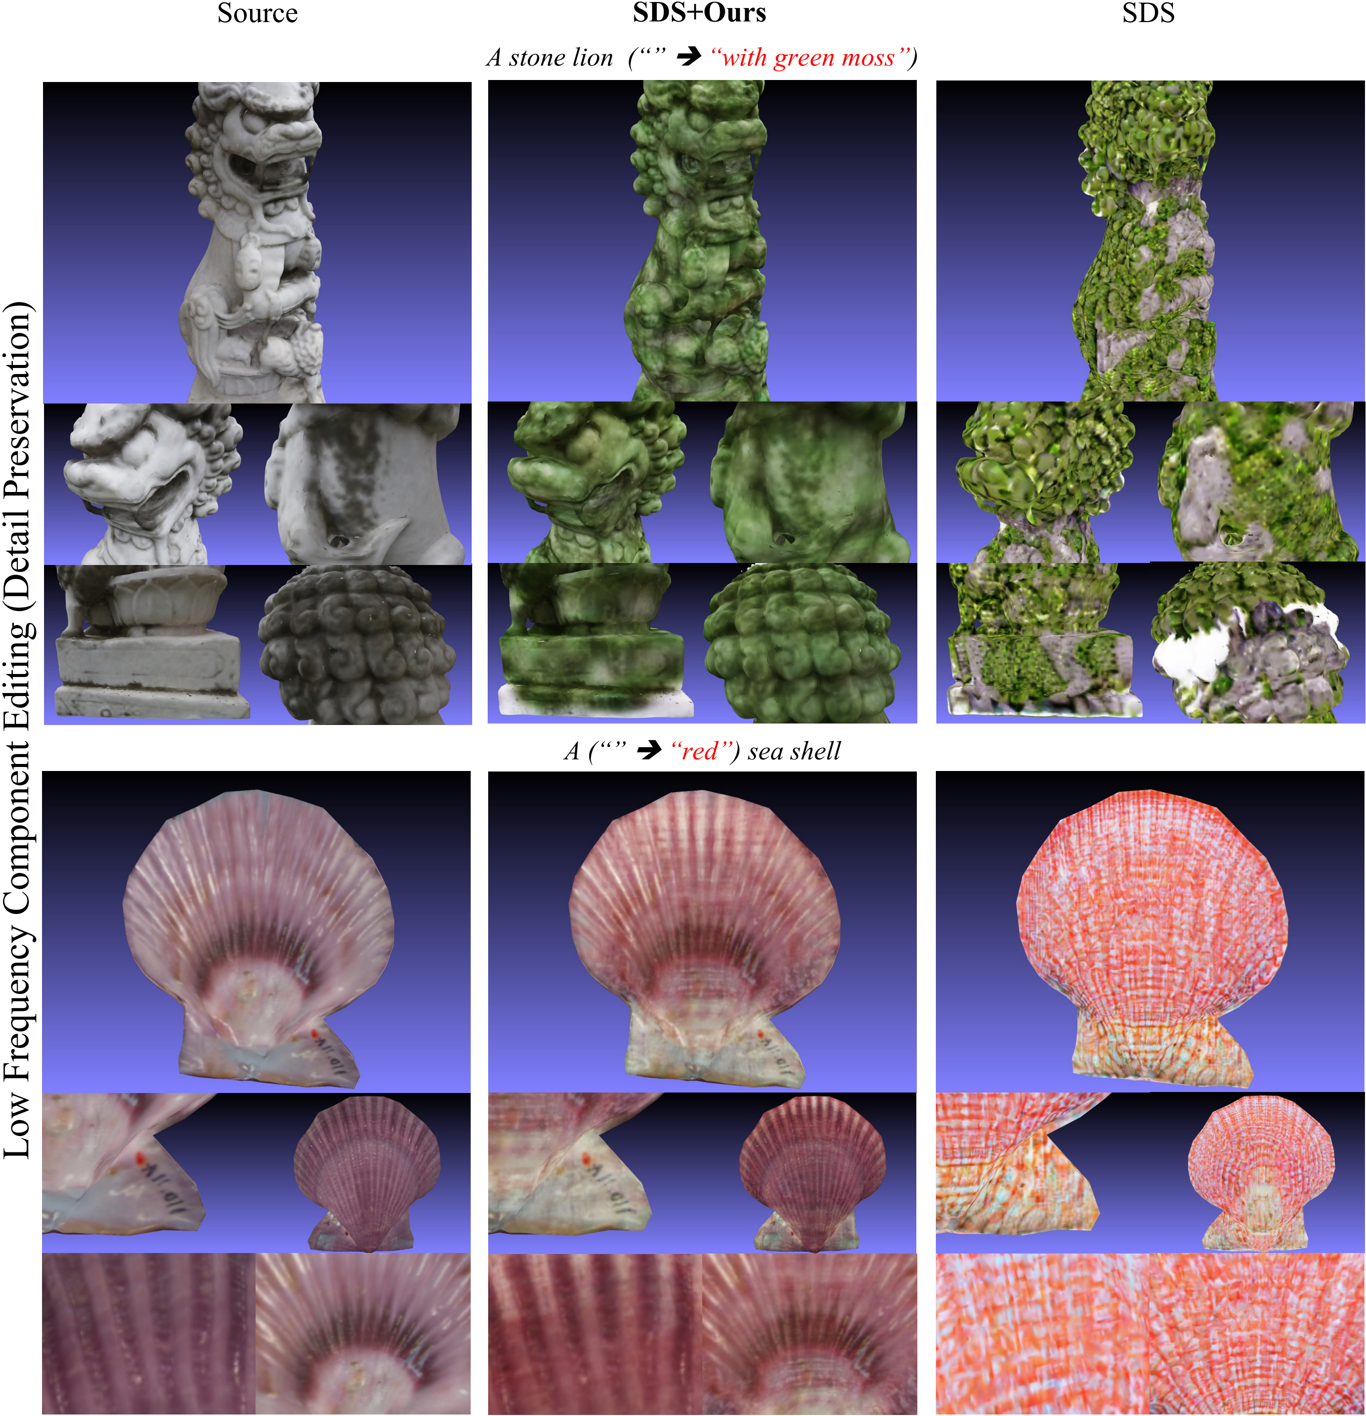

Source
SDS+Ours
SDS
A stone lion (“” ➔ “with green moss”)
A (“” ➔ “red”) sea shell
Low Frequency Component Editing (Detail Preservation)

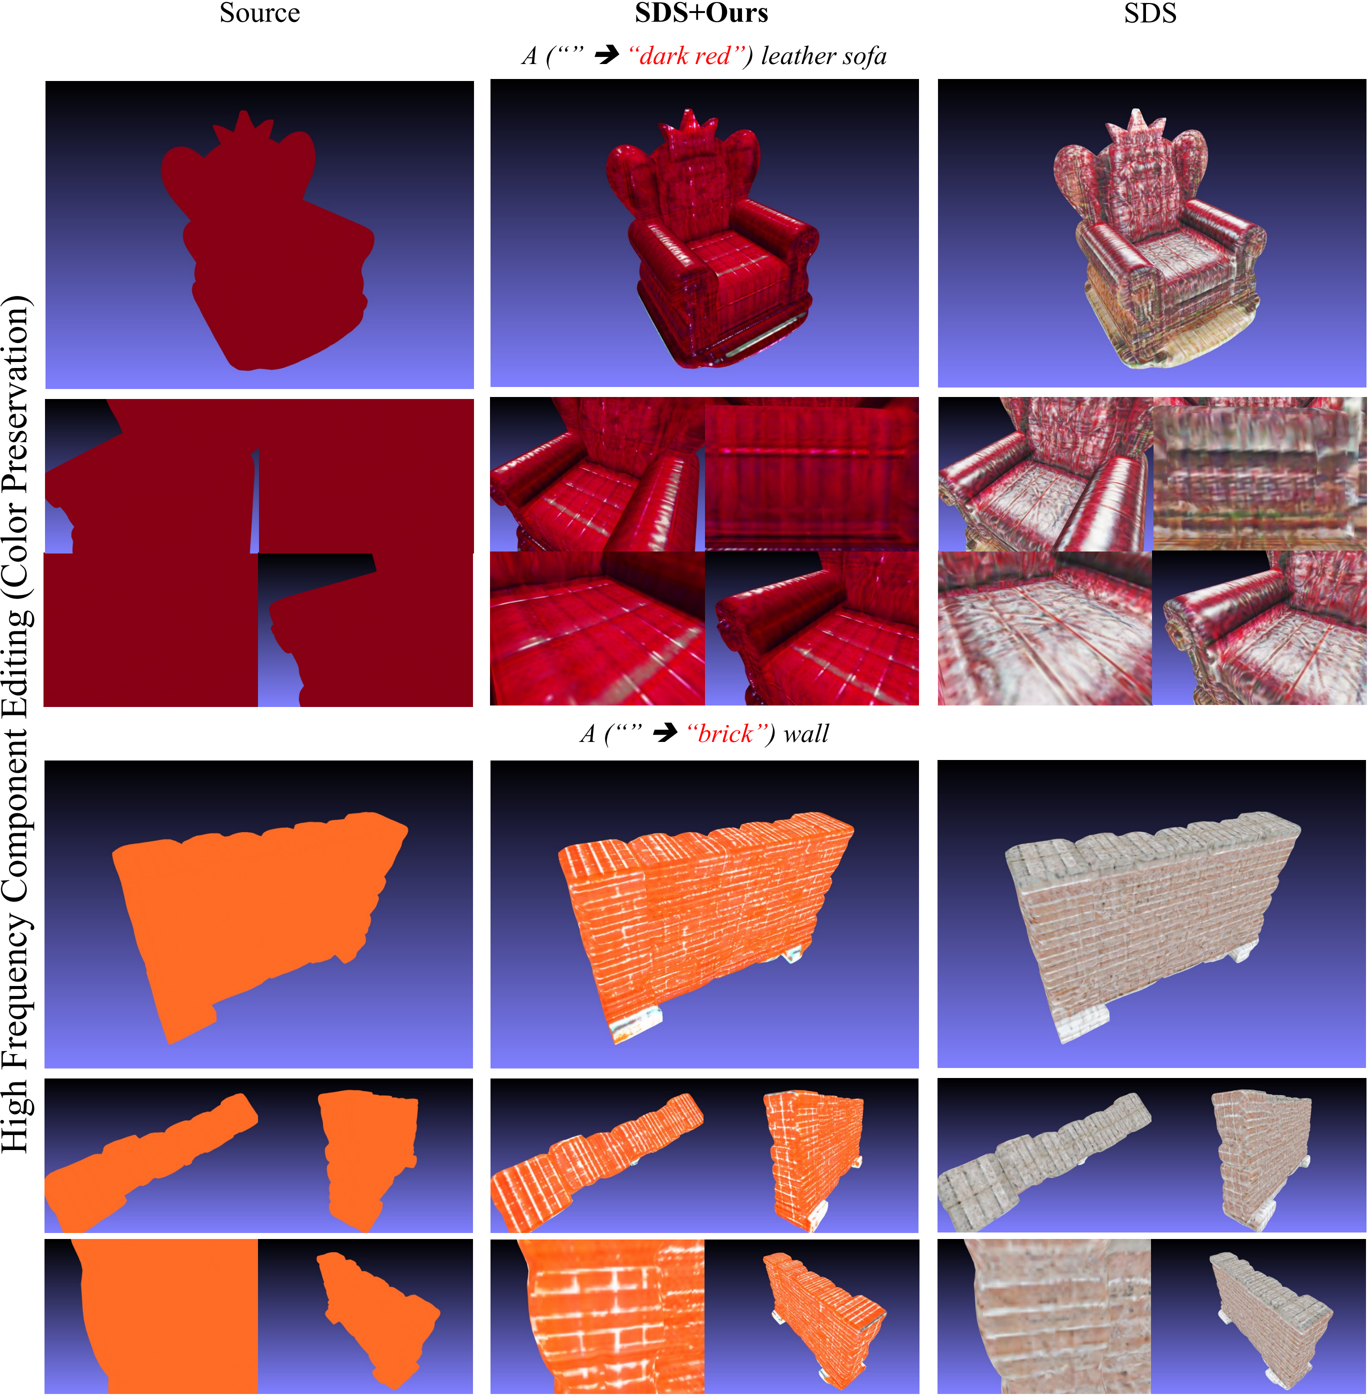
Source
SDS+Ours
SDS
A (“” ➔ “dark red”) leather sofa
A (“” ➔ “brick”) wall
High Frequency Component Editing (Color Preservation)

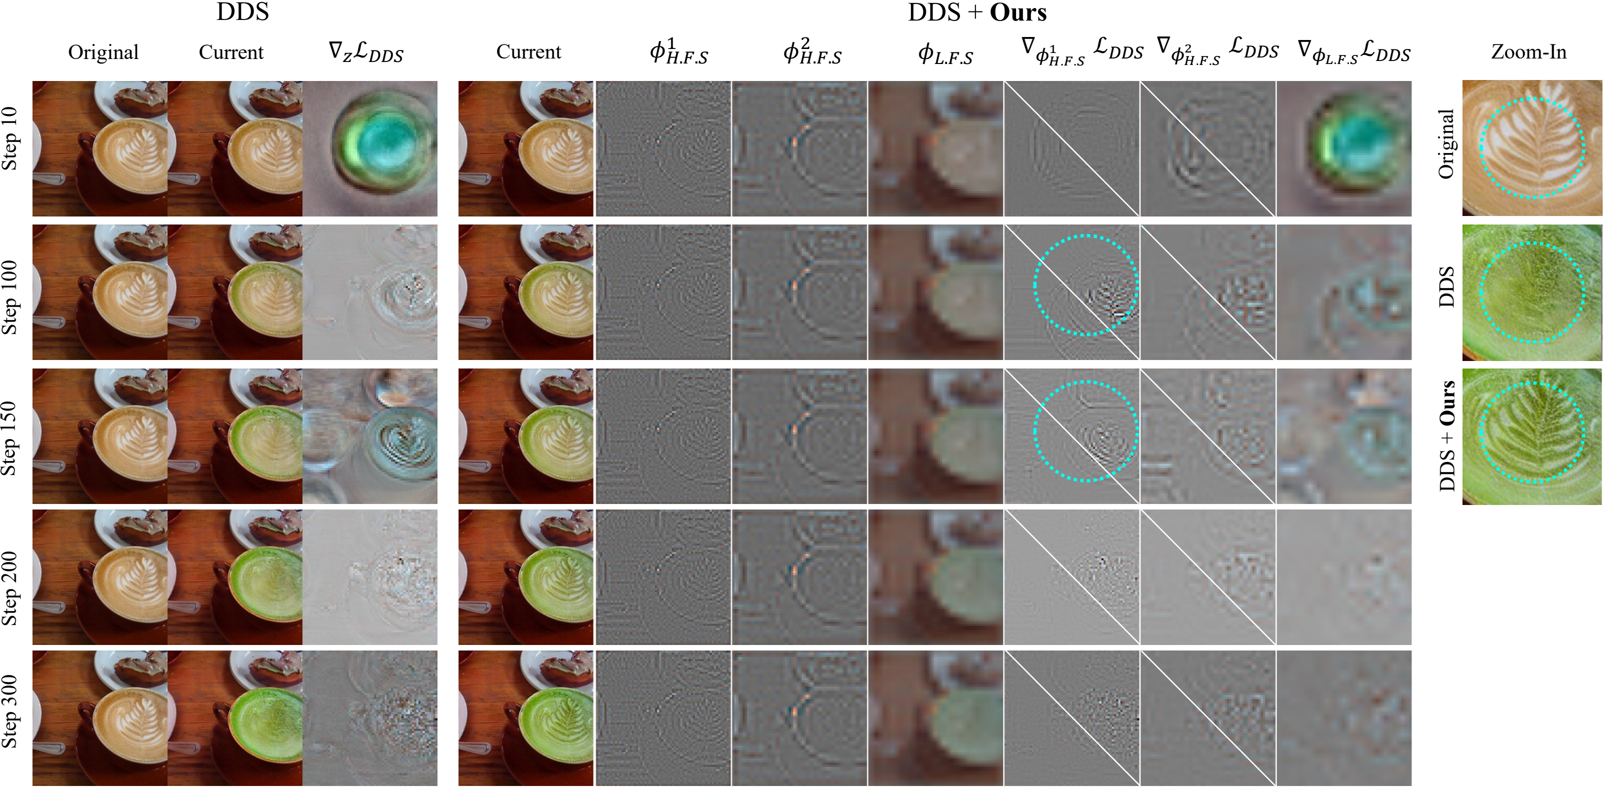

DDS
DDS + Ours
Original
Current
$\nabla_z \mathcal{L}_{DDS}$
Current
$\phi^1_{H.F.S}$
$\phi^2_{H.F.S}$
$\phi_{L.F.S}$
$\nabla_{\phi^1_{H.F.S}} \mathcal{L}_{DDS}$
$\nabla_{\phi^2_{H.F.S}} \mathcal{L}_{DDS}$
$\nabla_{\phi_{L.F.S}} \mathcal{L}_{DDS}$
Zoom-In
Step 10
Step 100
Step 150
Step 200
Step 300
Original
DDS
DDS + Ours

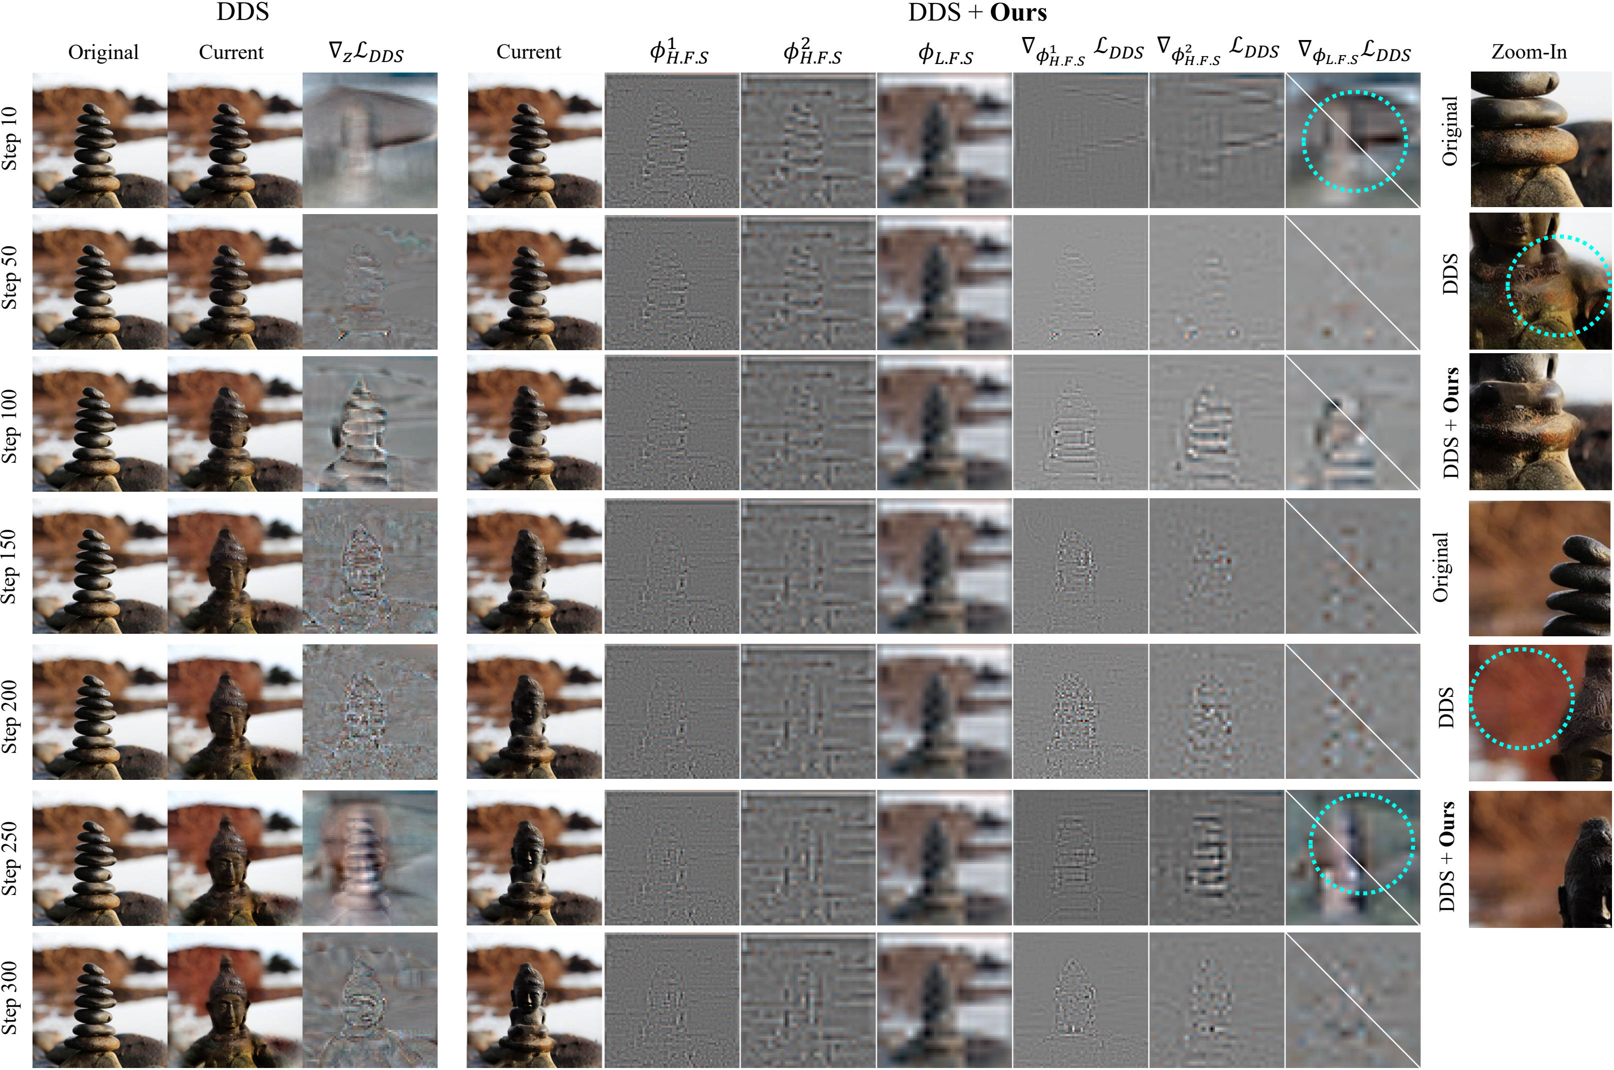
DDS
DDS + Ours
Original
Current
$\nabla_z \mathcal{L}_{DDS}$
Current
$\phi^1_{H.F.S}$
$\phi^2_{H.F.S}$
$\phi_{L.F.S}$
$\nabla_{\phi^1_{H.F.S}} \mathcal{L}_{DDS}$
$\nabla_{\phi^2_{H.F.S}} \mathcal{L}_{DDS}$
$\nabla_{\phi_{L.F.S}} \mathcal{L}_{DDS}$
Zoom-In
Step 10
Step 50
Step 100
Step 150
Step 200
Step 250
Step 300
Original
DDS
DDS + Ours
Original
DDS
DDS + Ours

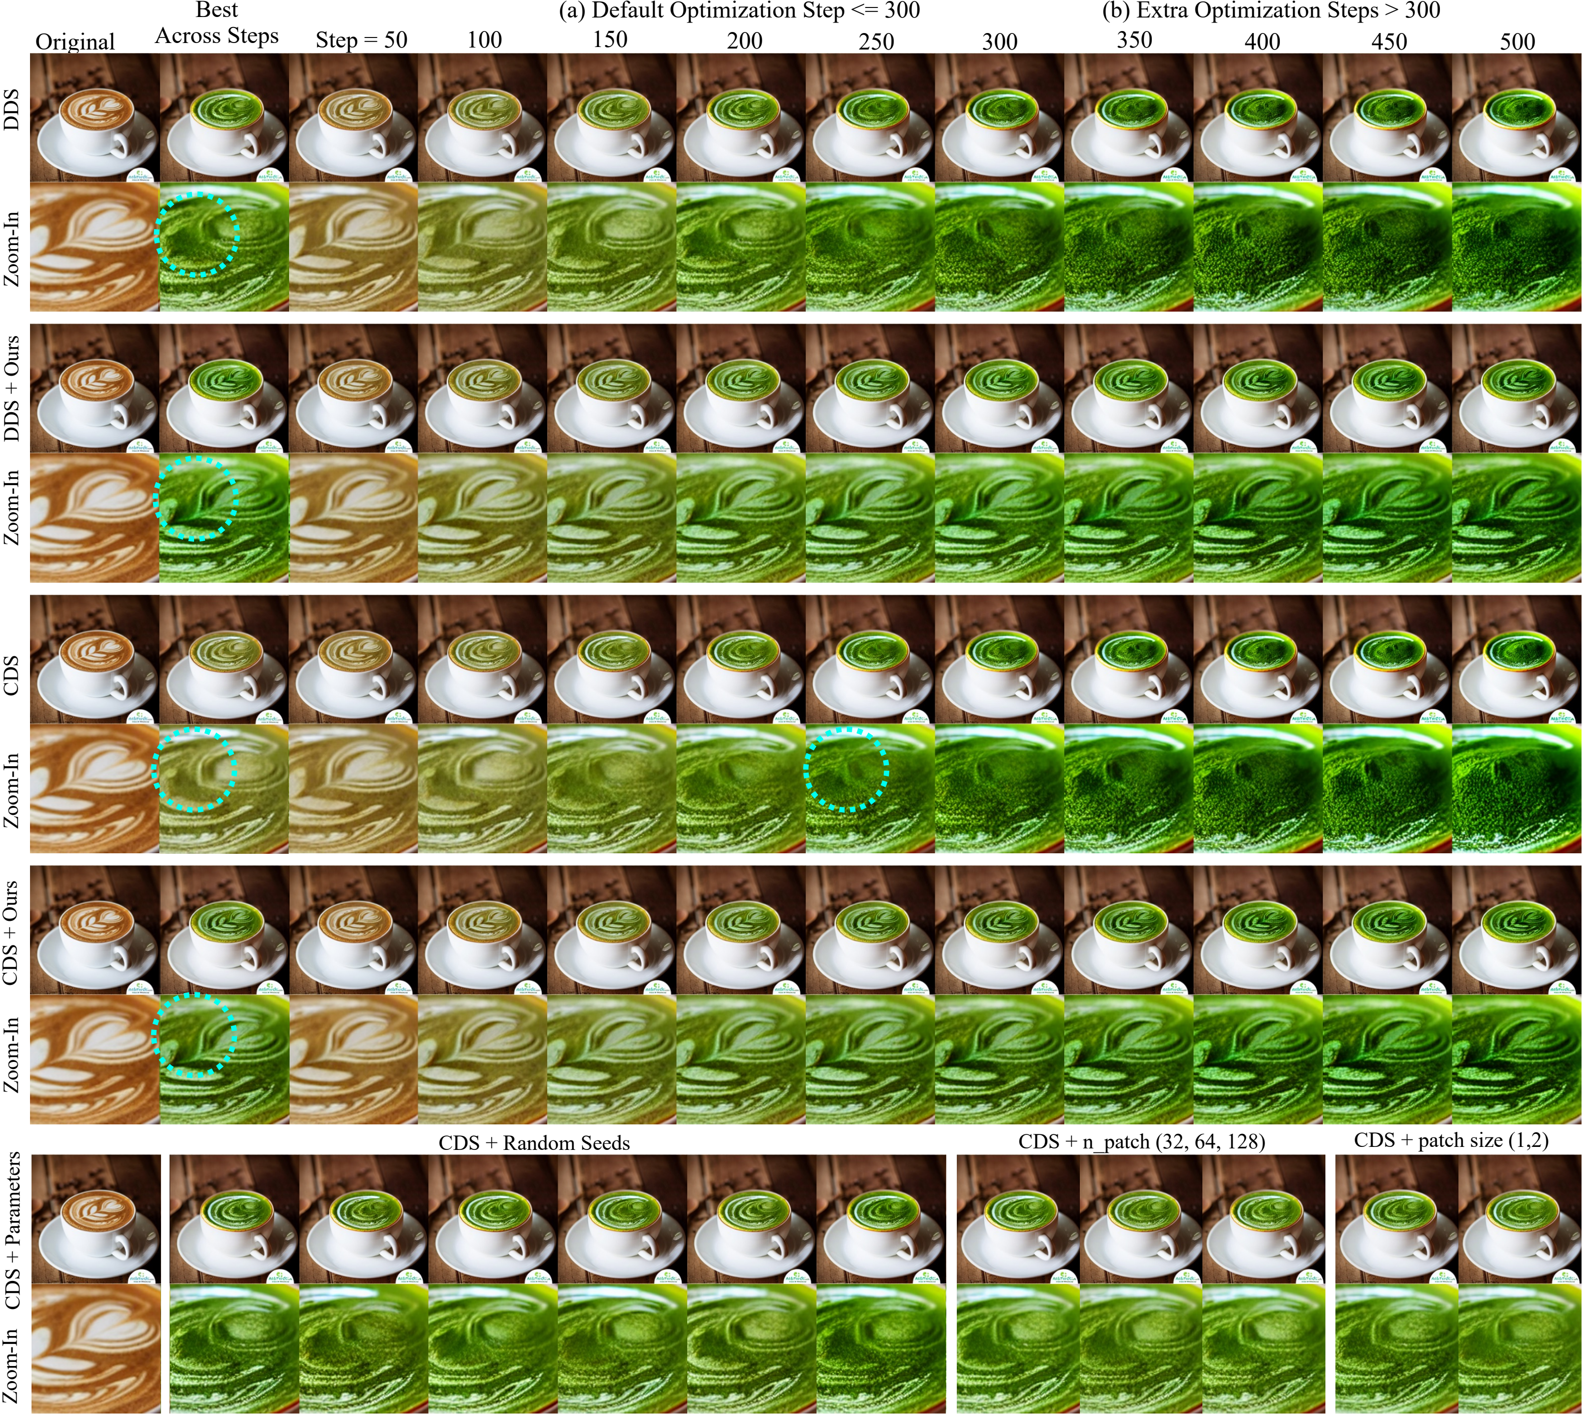
Original
Best Across Steps
(a) Default Optimization Step <= 300
Step = 50
100
150
200
250
300
(b) Extra Optimization Steps > 300
350
400
450
500
DDS
Zoom-In
DDS + Ours
Zoom-In
CDS
Zoom-In
CDS + Ours
Zoom-In
CDS + Parameters
Zoom-In
CDS + Random Seeds
CDS + n_patch (32, 64, 128)
CDS + patch size (1,2)
