# Supplementary material for: FDS: Frequency-Aware Denoising Score for Text-Guided Latent Diffusion Image Editing
Source: arXiv:2503.19191 source file (2025-03-24)
Supplement: Supplementary file 2 [file figs-supp2.pdf]

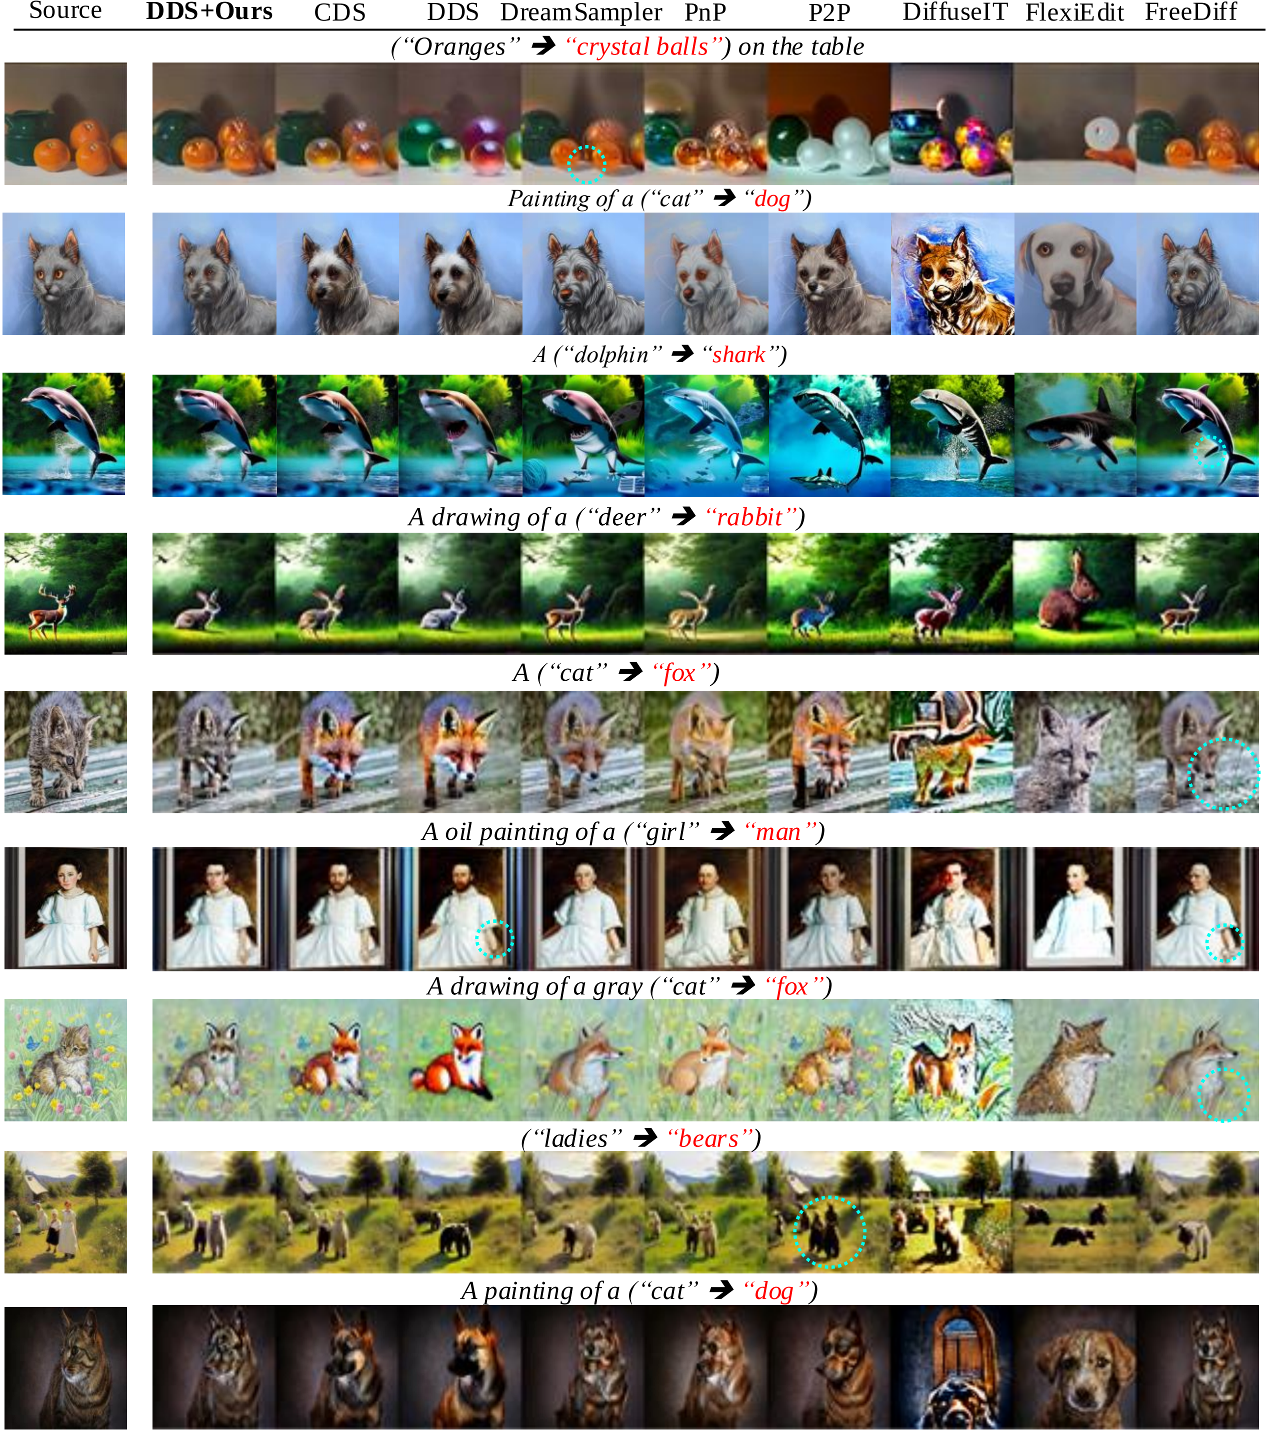
Source
DDS+Ours
CDS
DDS
DreamSampler
PnP
P2P
DiffuseIT
FlexiEdit
FreeDiff
("Oranges" ➔ "crystal balls") on the table
Painting of a ("cat" ➔ "dog")
A ("dolphin" ➔ "shark")
A drawing of a ("deer" ➔ "rabbit")
A ("cat" ➔ "fox")
A oil painting of a ("girl" ➔ "man")
A drawing of a gray ("cat" ➔ "fox")
("ladies" ➔ "bears")
A painting of a ("cat" ➔ "dog")

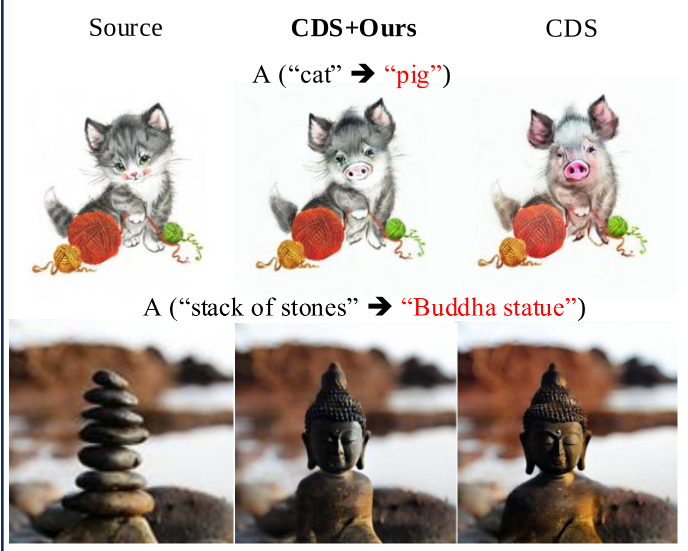


(a) Combining ours with CDS

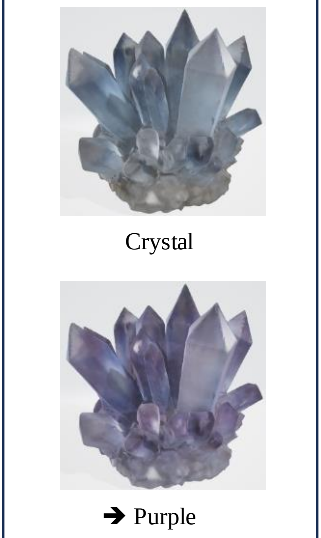


(b) Self-Occlusion

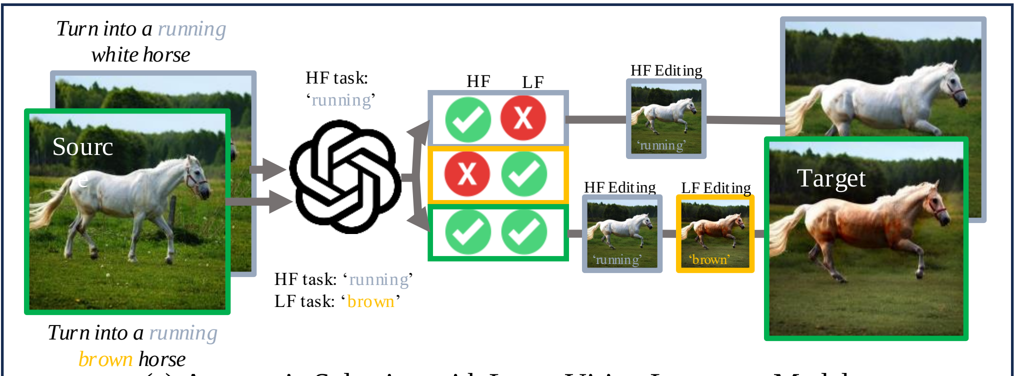


(c) Automatic Selection with Large Vision Language Models

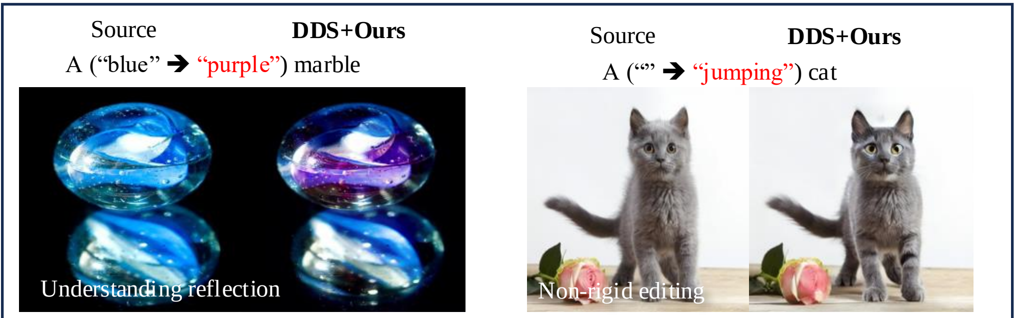


(d) Failure Cases

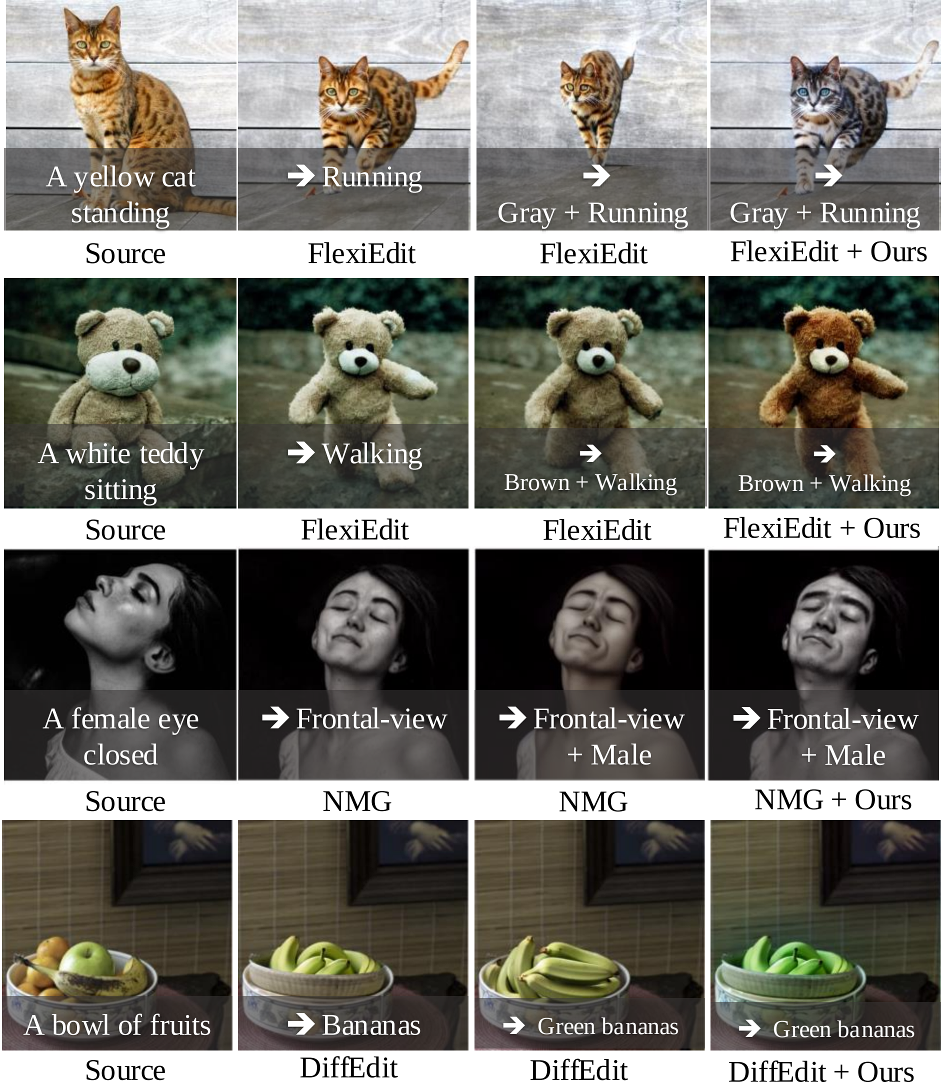
A yellow cat standing
➔ Running
➔ Gray + Running
➔ Gray + Running
Source
FlexiEdit
FlexiEdit
FlexiEdit + Ours
A white teddy sitting
➔ Walking
➔ Brown + Walking
➔ Brown + Walking
Source
FlexiEdit
FlexiEdit
FlexiEdit + Ours
A female eye closed
➔ Frontal-view
➔ Frontal-view + Male
➔ Frontal-view + Male
Source
NMG
NMG
NMG + Ours
A bowl of fruits
➔ Bananas
➔ Green bananas
➔ Green bananas
Source
DiffEdit
DiffEdit
DiffEdit + Ours
